# Supplementary material for: An Approach to Regular Separability in Vector Addition Systems
Source: arXiv:2007.00111 source file (2020-06-30)
Supplement: Supplementary file 1 [file appendix-results.tex]

% !TEX root = main.tex
\subsection{Proof of \cref{sepcartesian}}
In our proof of \cref{sepcartesian}, we use a well-known fact about
regular separability of unions.
\begin{lemma}\label{finiteunions}
  Let $X=\bigcup_{i=1}^n X_i$ and $Y=\bigcup_{j=1}^m Y_j$ for subsets
  $X,Y\subseteq M$.  Then $\sep{X}{Y}$ if and only if $\sep{X_i}{Y_j}$
  for every $i\in[1,n]$ and $j\in[1,m]$.
\end{lemma}
\begin{proof}
  A separator witnessing $\sep{X}{Y}$ also witnesses $\sep{X_i}{Y_j}$
  for every $i\in[1,n]$ and $j\in[1,m]$. This shows the ``only if'' direction.

  For the ``if'' direction, suppose $R_{i,j}\subseteq M$ satisfies
  $X_i\subseteq R_{i,j}$ and $R_{i,j}\cap Y_j=\emptyset$. We claim that
  $R=\bigcup_{i=1}^n \bigcap_{j=1}^m R_{i,j}$ witnesses $\sep{X}{Y}$.

  Since $X_i\subseteq R_{i,j}$ for every $i\in[1,n]$, we have
  $X_i\subseteq\bigcap_{j=1}^m R_{i,j}$ and hence
  $X=\bigcup_{i=1}^n X_i\subseteq R$. On the other hand, for every $i\in[1,n]$ and $k\in[1,m]$,
  we have $Y_k\cap R_{i,k}=\emptyset$ and thus $Y_k\cap \bigcap_{j=1}^m R_{i,j}=\emptyset$.
  This implies 
  \[ Y\cap R=\bigcup_{k=1}^m Y_k\cap \bigcup_{i=1}^n\bigcap_{j=1}^m R_{i,j}=\bigcup_{k=1}^m \bigcup_{i=1}^n \underbrace{Y_k\cap \bigcap_{j=1}^m R_{i,j}}_{=\emptyset}=\emptyset. \]
\end{proof}

\begin{proof}[Proof of \cref{sepcartesian}]
One direction is immediate: If $\sep{X}{Y}$ with a recognizable separator $S\subseteq
M$, then $X\times Y$ is separated from $\Delta$ by the recognizable set
$S\times (M\setminus S)$.

Suppose $\sep{(X\times Y)}{\Delta}$ is witnessed by $S\subseteq M\times M$ with $X\times
Y\subseteq S$ and $S\cap\Delta=\emptyset$. We can write $S=\bigcup_{i=1}^n
R_i\times T_i$ for recognizable subsets $R_i,T_i\subseteq M$ for $i\in[1,n]$~\cite{Ber79}.
Note that then $(R_i\times T_i)\cap\Delta=\emptyset$ and thus $T_i\subseteq
M\setminus R_i$. Moreover, we have $X\subseteq \bigcup_{i=1}^n R_i$ and
$Y\subseteq \bigcup_{i=1}^n T_i\subseteq \bigcup_{i=1}^n (M\setminus R_i)$.

For any $I\subseteq [1,n]$,
\todo{Reviewer wanted to rewrite this paragraph. I see nothing wrong here. Georg: Add some more explanation.}
let $R_I=\bigcap_{i\in I} R_i\cap
\bigcap_{i\in[1,n]\setminus I} (M\setminus R_i)$, $X_I=X\cap R_I$, and
$Y_I=Y\cap R_I$. We claim that for any $I,J\subseteq [1,n]$, we have
$X_I|Y_J$. Since $X=\bigcup_{\emptyset\ne I\subseteq [1,n]} X_I$ and
$Y=\bigcup_{I\subsetneq [1,n]} Y_I$, the \lcnamecref{sepcartesian}
then follows from \cref{finiteunions}.

Suppose $I=J$. We shall prove that then either $X_I=\emptyset$ or
$Y_J=\emptyset$, which clearly implies $\sep{X_I}{Y_J}$. Toward a contradiction,
assume that there are $x\in X_I$ and $y\in Y_J$. Since $X\times Y\subseteq S$,
there is an $i\in[1,n]$ with $x\in R_i$ and $y\in T_i\subseteq (M\setminus
R_i)$. The former implies $i\in I$, and the latter $i\notin J$, contradicting
$I=J$.

Suppose $I\ne J$. If there is an $i\in I\setminus J$, then $X_I\subseteq
R_I\subseteq R_i$ and $Y_J\subseteq R_J\subseteq M\setminus R_i$, meaning that
$R_i$ witnesses $\sep{X_I}{Y_J}$. On the other hand, if $i\in J\setminus I$, then
$X_I\subseteq M\setminus R_i$ and $Y_J\subseteq R_i$, so that $M\setminus R_i$
witnesses $\sep{X_I}{Y_J}$.
%We claim that the set
%\[ S' = \bigcup_{I\subseteq [1,n],~X\cap R_I\ne\emptyset} R_I \]
%separates $X$ from $Y$. Clearly, since $X\subseteq \bigcup_{i=1} R_i$, each
%$x\in X$ has a non-empty set $I_x=\{i\in[1,n] \mid x\in R_i\}$. Hence, $x\in
%R_{I_x}\subseteq S'$. Furthermore, if there is a $y\in Y\cap S'$, then $y\in
%R_I$ for some $I\subseteq [1,n]$ with $X\cap R_I\ne\emptyset$. This means there
%is an $x\in X\cap R_I$. However, $(x,y)\in X\times Y\subseteq S$ and hence 
\end{proof}

%%% Local Variables:
%%% mode: latex
%%% TeX-master: "main"
%%% End:
