# Supplementary material for: An Approach to Regular Separability in Vector Addition Systems
Source: arXiv:2007.00111 source file (2020-06-30)
Supplement: Supplementary file 2 [file appendix-vass-comm.tex]

For $\vec u,\vec v\in\N^\Sigma$ and $k\in\N$, let
$\vec u\vequiv_k \vec v$ if for every $k$-state DFA $\cA$, we have
$\Parikh^{-1}(u)\subseteq\Lang{\cA}$ if and only if
$\Parikh^{-1}(\vec v)\subseteq\Lang{\cA}$. Note that for each
$k\in\N$, $\vequiv_k$ is an equivalence relation of finite index.

For $w\in\Sigma^*$ and $\vec u\in\N^\Sigma$, we write $w\wvequiv_k u$
if for every $k$-state DFA $\cA$, the inclusion
$\Parikh^{-1}(\vec u)\subseteq\Lang{\cA}$ implies $w\in\Lang{\cA}$.
For a language $L\subseteq\Sigma^*$ and a set $U\subseteq\N^\Sigma$,
we say that a sequence $(w_1,\vec u_1),(w_2,\vec u_2),\ldots$ is an
$(L,U)$-chain if $w_k\in L$ and $\vec u_k\in U$ and
$w_k\wvequiv \vec u_k$ for every $k\ge 1$.
\begin{lemma}
  Let $L\subseteq\Sigma^*$ and $U\subseteq\N^\Sigma$. Then
  $\sep{L}{\Parikh^{-1}(U)}$ if and only if there is no $(L,U)$-chain.
\end{lemma}
\begin{proof}
  Suppose there is no $(L,U)$-chain. Then there is a number $k\in\N$
  such that there is no pair $(w,\vec u)\in L\times U$ with
  $w \wvequiv_k \vec u$. In order to show that
  $\sep{L}{\Parikh^{-1}(U)}$, we show that every
  $\vequiv_k$-equivalence class $C$ that intersects $U$ has the
  property $\sep{L}{\Parikh^{-1}(C)}$. Since there are only finitely
  many such classes, this implies $\sep{L}{\Parikh^{-1}(U)}$.
  
  Consider such a class $C$ with a representative $\vec u\in C\cap U$.
  Let $R\subseteq\Sigma^*$ be the intersection of all $\Lang{\cA}$,
  where $\cA$ is a $k$-state DFA with
  $\Parikh^{-1}(C)\subseteq\Lang{\cA}$. Since there are only finitely
  many $k$-state DFAs, $R$ is a regular language. Then clearly
  $\Parikh^{-1}(C)\subseteq R$ and we have to check that
  $R\cap L=\emptyset$. Suppose there is a $w\in L$ with $w\in R$. Then
  for every $k$-state DFA $\cA$ with
  $\Parikh^{-1}(C)\subseteq\Lang{\cA}$, we have
  $w\in\Lang{\cA}$. Since $C$ is the $\vequiv_k$ equivalence class of
  $\vec u$, this means for every $k$-state DFA $\cA$ with
  $\Parikh^{-1}(\vec u)\subseteq\Lang{\cA}$, we have
  $w\in \Lang{\cA}$. This means $w\wvequiv_k \vec u$, which is impossible.
  Therefore, $R\cap L=\emptyset$ and hence $\sep{L}{\Parikh^{-1}(C)}$.

  Now suppose that $\sep{L}{\Parikh^{-1}(U)}$. Then there is a DFA
  $\cA$ with $\Parikh^{-1}(U)\subseteq\Lang{\cA}$ and
  $L\cap\Lang{\cA}=\emptyset$. If $k$ is the number of states in
  $\cA$, then this means for every $\vec u\in U$, there cannot be a
  $w\in L$ with $w\wvequiv_k \vec u$. In particular, an $(L,U)$ chain
  cannot exist.
\end{proof}

\begin{proposition}
  Let $L\subseteq\Sigma^*$ and let $U\subseteq\N^\Sigma$ be a VASS
  section. Then $\sep{L}{\Parikh^{-1}(U)}$ if and only if for every
  semilinear $S\subseteq U$, we have $\sep{L}{\Parikh^{-1}(S)}$.
\end{proposition}
\begin{proof}
  The ``only if'' direction is immediate. For the ``if'' direction,
  suppose that $\sep{L}{\Parikh^{-1}(U)}$ does not hold. Then there is
  an $(L,U)$ chain $(w_1,\vec u_1),(w_2,\vec u_2),\ldots$. For each
  $i\ge 1$, let $\rho_i$ be a run of the VASS for $U$ such that
  $\rho_i$ reads a word with image $\vec u_i$. By picking a
  subsequence, we may assume that $\rho_1\unlhd\rho_2\unlhd\cdots$.
  We call $a\in\Sigma$ \emph{bounded} if the number sequence
  $\vec u_1(a), \vec u_2(a),\ldots$ is bounded. By removing some
  initial segment of our $(L,U)$ chain, we may assume that for every
  bounded $a\in\Sigma$, we have $\vec u_1(a)=\vec u_2(a)=\cdots$.

  Consider the set $D=\{\vec u_i-\vec u_1 \mid i\ge 1\}$ of
  differences and the subgroup of $G$ of $\Z^\Sigma$ generated by
  $D$. As a subgroup of a finitely generated free abelian group, $G$
  is finitely generated, say by
  $P=\{\vec u_{i_1}-\vec u_1,\ldots,\vec u_{i_m}-\vec u_1\}$.
  Let $S=\vec u_1+\linspan_\N P$. %FIXME finish
\end{proof}
%%% Local Variables:
%%% mode: latex
%%% TeX-master: "main"
%%% End:
